# Supplementary material for: Atomic Learning Objectives Labeling: A High-Resolution Approach for Physics Education
Source: arXiv:2412.09914 source file (2025-02-22)
Supplement: Supplementary file 2 [file appendix_examples_math.tex]

\begin{table*}[t!]
\centering
\begin{minipage}[t]{1\textwidth}
\begin{lstlisting}[mathescape=true,basicstyle=\ttfamily\smalltonormalsize]
$\textbf{Math Question Set Example 1}$: 

Content Classification: Number & Operation
            
Question: What number is subtracted from 1,000 to result in a difference of 421?

Answer and Rationales:
$\colorbox{lightyellow}{A: 421}$
Rationale A: Selects the result of subtraction.
$\colorbox{lightyellow}{B: 579}$
Rationale B: 1000 - 421 = 579
$\colorbox{lightyellow}{C: 621}$
Rationale C: Rounded the hundreds place and added the tens and ones place. 1000 - 400 = 600; 600 + 21 = 621
$\colorbox{lightyellow}{D: 689}$
Rationale D: Rounded in hundreds, tens and ones place. 1000 - 400 = 600; 100 - 20 = 80; 10 - 1 = 9; 600 + 80 + 9 = 689

$\textbf{Math Question Set Example 2}$: 

Content Classification: Algebra
            
Question: Anne bought a calculator that cost 30. She received 10% off her purchase and then was charged 6% tax. What was the total amount that Anne paid?

Answer and Rationales:
$\colorbox{lightyellow}{A: 21.20}$
Rationale A: Subtracted 10 from 30, then added 6%.
$\colorbox{lightyellow}{B: 25.38}$
Rationale B: Subtracted 10% of the price from 30 then subtracted 6%.
$\colorbox{lightyellow}{C: 28.62}$
Rationale C: Subtracted 10% of the price from 30 and then added 6%.
$\colorbox{lightyellow}{D: 28.80}$
Rationale D: Calculated tax based on original price, then subtracted the 3.

$\textbf{Math Question Set Example 3}$: 

Content Classification: Geometry and Measurement
            
Question: Which side lengths form a right triangle?

Answer and Rationales:
$\colorbox{lightyellow}{A: 2 cm, 4 cm, 8 cm}$
Rationale A: Multiplied the 2 smaller sides to get the longest side.
$\colorbox{lightyellow}{B: 4 cm, 5 cm, 6 cm}$
Rationale B: Selected side with constant difference between the sides.
$\colorbox{lightyellow}{C: 5 cm, 12 cm, 13 cm}$
Rationale C: 5^2 + 12^2 = 13^2
$\colorbox{lightyellow}{D: 9 cm, 16 cm, 25 cm}$
Rationale D: Added the 2 smaller sides to get the longest side.

	
\end{lstlisting}
\end{minipage}
\hfill
\caption{Examples of Mathematics question set. }
\label{tab:math_example-1}
\end{table*}

\begin{table*}[t!]
\centering
\begin{minipage}[t]{1\textwidth}
\begin{lstlisting}[mathescape=true,basicstyle=\ttfamily\smalltonormalsize]
$\textbf{Math Question Set Example 4}$: 

Content Classification: Data Analysis
            
Question: Mrs. Castillo recorded the number of students in each grade 5 classroom.
            24  28  25  24  29
What is the mean of the data?

Answer and Rationales:
$\colorbox{lightyellow}{A: 24}$
Rationale A: Chose the mode.
$\colorbox{lightyellow}{B: 25}$
Rationale B: Chose the median. {24, 24, 25, 28, 29}
$\colorbox{lightyellow}{C: 26}$
Rationale C: (24 + 28 + 25 + 24 + 29) / 5 = 130/5 = 26
$\colorbox{lightyellow}{D: 29}$
Rationale D: Chose the greatest number.

$\textbf{Math Question Set Example 5}$: 

Content Classification: Probability
            
Question: Ms. Collier had a deck of cards. There were stars on 1/4 of the cards in the deck. After randomly picking a card and returning it to the deck 100 times, the expected result and relative frequency of picking a card with a star were equal. In the first 50 cards she picked, she got a star 10 times. How many times did Ms. Collier get a star in the second 50 cards she picked?

Answer and Rationales:
$\colorbox{lightyellow}{A: 10}$
Rationale A: Chose the number of times a star is picked in the 1st 50 cards drawn.
$\colorbox{lightyellow}{B: 13}$
Rationale B: Calculated 50 * 1/4 = 12.5 and then rounded to 13.
$\colorbox{lightyellow}{C: 15}$
Rationale C: Correct. 100 * 1/4 = 25 cards w/ stars. 25 - 10 = 15
$\colorbox{lightyellow}{D: 25}$
Rationale D: Calculated 100 * 1/4 = 25 cards w/ stars.

	
\end{lstlisting}
\end{minipage}
\hfill
\caption{Examples of Mathematics question set. }
\label{tab:math_example-2}
\end{table*}
